# Supplementary material for: Constructing hierarchical time series through clustering: Is there an optimal way for forecasting?
Source: arXiv:2404.06064 source file (2024-09-08)
Supplement: Supplementary file 1 [file supplementary.pdf]

# Supplementary material

This supplementary material provides results on forecast performance of middle-level series defined by the natural hierarchy. For cluster hierarchies and two-level hierarchies where these middle-level series do not exist, we compute the middle-level forecasts using a bottom-up strategy. The average RMSSE based on different approaches for the tourism and mortality datasets are presented in Table S.1. The MCB test results on middle-level series are shown in Figure S.1.

Table S.1: Performance of all approaches in terms of average RMSSE across all evaluation windows on both datasets. Column-wise minimum values are displayed in bold. "Middle" refers to middle-levels defined by the natural hierarchy.

| Approach | tourism | | | mortality | | |
|---|---|---|---|---|---|---|
| | Top | Middle | Bottom | Top | Middle | Bottom |
| Base | **0.869** | 0.732 | 0.694 | 0.761 | 0.744 | 0.753 |
| Two-level | 0.923 | 0.730 | 0.694 | 0.736 | 0.735 | 0.753 |
| Natural | 0.876 | **0.717** | 0.691 | 0.738 | 0.732 | 0.750 |
| Grouped | 0.831 | 0.721 | 0.706 | 0.798 | 0.783 | 0.750 |
| TS-EUC-ME | 0.900 | 0.727 | 0.693 | 0.728 | 0.735 | 0.753 |
| ER-EUC-ME | 0.918 | 0.727 | 0.693 | 0.741 | 0.740 | 0.753 |
| TSF-EUC-ME | 0.907 | 0.728 | 0.693 | 0.739 | 0.741 | 0.755 |
| ERF-EUC-ME | 0.909 | 0.729 | 0.694 | 0.733 | 0.738 | 0.753 |
| TS-EUC-HC | 0.874 | 0.719 | 0.692 | 0.740 | 0.730 | 0.754 |
| ER-EUC-HC | 0.890 | 0.719 | 0.691 | 0.746 | 0.732 | 0.751 |
| TSF-EUC-HC | 0.881 | 0.719 | 0.690 | 0.744 | 0.739 | 0.751 |
| TS-DTW-ME | 0.909 | 0.729 | 0.693 | **0.726** | 0.734 | 0.753 |
| TS-DTW-HC | 0.878 | 0.719 | 0.691 | 0.731 | 0.730 | 0.750 |
| ER-DTW-ME | 0.911 | 0.729 | 0.694 | 0.733 | 0.739 | 0.753 |
| ER-DTW-HC | 0.878 | 0.719 | 0.691 | 0.748 | 0.736 | 0.753 |
| Combination | 0.893 | 0.721 | **0.690** | 0.730 | **0.724** | **0.725** |

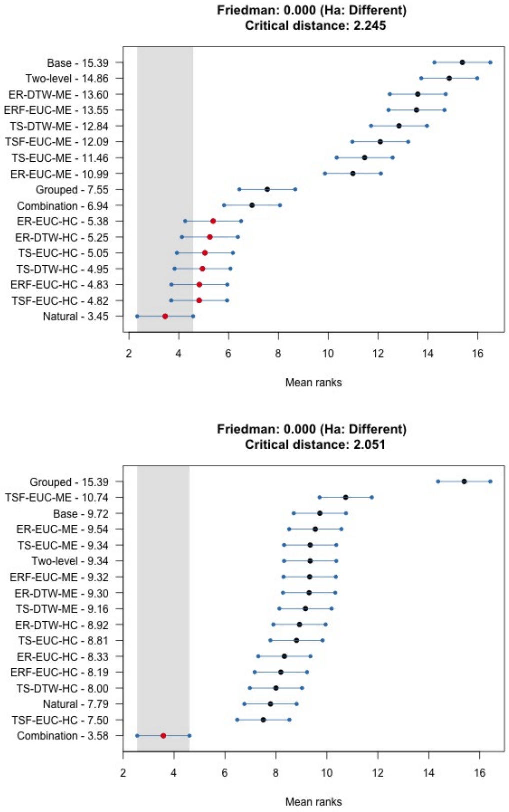


Figure S.1: Average ranks and 95% confidence intervals for all approaches on middle level of tourism dataset (left) and mortality dataset (right) based on MCB test.
